# Supplementary material for: PSC-CPI: Multi-Scale Protein Sequence-Structure Contrasting for Efficient and Generalizable Compound-Protein Interaction Prediction
Source: arXiv:2402.08198 source file (2024-02-13)
Supplement: Supplementary file 1 [file appendix.tex]

\setcounter{table}{0}
\setcounter{figure}{0}

\section*{Appendix}

\subsection*{A. Pseudo-Code}
Taking multimodal inference with protein sequences and structures as an example, the pseudo-code for pre-training, fine-tuning, and inference is summarized in Algorithm~\ref{algo:1}.

\begin{algorithm}[!htbp]
	\caption{Algorithm for CPI Prediction (Multimodal)}
	\label{algo:1}
	\begin{algorithmic}[1]
		\Require Compound Graphs $\{\mathcal{G}_C^{(j)}\}_{j=1}^M$, Protein Sequences $\{S^{(i)}\}_{i=1}^N$, and Protein Graphs $\{\mathcal{G}_{\mathcal{P}}^{(i)}\}_{i=1}^N$.
  	\Ensure Interaction pattern $\mathbf{P}^{\text{cont}}$ and strength $y^{\text{aff}}$.

        \State \# \textit{Pre-training}
         \While{\textit{not convergence}}
            \State Generate a set of subsequences and subgraphs by ${\color[rgb]{1.0, 1.0, 1.0}AA}$ length-variable augmentation;
            \State Pass the augmented subsequences and subgraphs  ${\color[rgb]{1.0, 1.0, 1.0}AA}$ through the sequence and structure encoders;
            \State Pre-train the two encoders by intra-modality and ${\color[rgb]{1.0, 1.0, 1.0}AA}$  cross-modality contrastive losses in Eq.~(\ref{eq:7})(\ref{eq:8})(\ref{eq:9}).
         \EndWhile

        \State \# \textit{Fine-tuning}
        \While{\textit{not convergence}}
		\State Jointly train the two pre-trained encoders and com- ${\color[rgb]{1.0, 1.0, 1.0}AA}$ pound encoder by loss in Eq.~(\ref{eq:10}) or (\ref{eq:11}).
        \EndWhile

        \State \# \textit{Inference}
        \State Predict interaction pattern $\mathbf{P}^{\text{cont}}$ and interaction strength $y^{\text{aff}}$ for any given compound-protein pair.
		\State \textbf{return}  Interaction pattern $\mathbf{P}^{\text{cont}}$ and strength $y^{\text{aff}}$.
	\end{algorithmic}
\end{algorithm}

\subsection*{B. Evaluation on More Metrics and Architectures}
We report the performance of CPI pattern prediction and strength prediction under four different test data splits on the Karimi dataset in Table.~\ref{tab:A1} and Table.~\ref{tab:A2}, respectively. For unimodal inference with only protein sequences or structures, HRNN, LSTM \cite{hochreiter1997long}, Bi-LSTM are considered as sequence encoders and GCN \cite{kipf2016semi}, GAT \cite{velivckovic2017graph}, SAGE \cite{hamilton2017inductive} are considered as structure encoders, respectively. For multimodal inference with both sequences and structures, we adopt HRNN as the sequence encoder and GAT as the structure encoder by default and consider two representation integrations, i.e., Concatenation and Cross Interaction \cite{you2022cross}. We can observe from Table.~\ref{tab:A1} and \ref{tab:A2} that PSC works well across various evaluation metrics and architectures.

\begin{table*}[!tbp]
\begin{center}
\caption{Performance comparison of \textit{CPI pattern prediction} with AUPRC (higher is better) and AUROC (higher is better) as evaluation metrics under four different data splits on the Karimi dataset, where three inference settings with different sequence and structure encoders are evaluated, respectively. The best metrics for each inference setting are marked by different colors.}
\label{tab:A1}
\resizebox{1.0\textwidth}{!}{
\begin{tabular}{clcccccccc}
\toprule
\multirow{2}{*}{\begin{tabular}[c]{@{}c@{}}\textbf{Inference} \textbf{Setting}\end{tabular}} & \multicolumn{1}{c}{\multirow{2}{*}{\textbf{Methods}}} & \multicolumn{2}{c}{\textbf{Seen-Both}} & \multicolumn{2}{c}{\textbf{Unseen-Comp}} & \multicolumn{2}{c}{\textbf{Unseen-Prot}} & \multicolumn{2}{c}{\textbf{Unseen-Both}} \\ \cmidrule(r){3-4}  \cmidrule(r){5-6} \cmidrule(r){7-8} \cmidrule(r){9-10}
 & \multicolumn{1}{c}{} & \textbf{AUPRC$\uparrow$} & \textbf{AUROC$\uparrow$} & \textbf{AUPRC$\uparrow$} & \textbf{AUROC$\uparrow$} & \textbf{AUPRC$\uparrow$} & \textbf{AUROC$\uparrow$} & \textbf{AUPRC$\uparrow$} & \textbf{AUROC$\uparrow$} \\ \midrule
\multirow{6}{*}{Sequence} & HRNN & 22.05 & 77.52 & 19.32 & 77.49 & 6.48 & 73.36 & 5.62 & 73.97 \\
 & pre-train w/ PSC & 22.29 & 77.68 & 21.43 & 78.09 & 7.01 & 75.36 & 6.64 & 74.77 \\ \cmidrule(r){2-10} 
 & LSTM & 20.88 & 77.30 & 20.15 & 77.98 & 5.68 & 73.72 & 5.60 & 71.93 \\
 & pre-train w/ PSC & 22.27 & 79.19 & 21.87 & 79.96 & 6.68 & 74.35 & 6.10 & 72.98 \\ \cmidrule(r){2-10} 
 & Bi-LSTM & 21.96 & 78.33 & 21.39 & 79.36 & 9.92 & 79.57 & \cellcolor{red!10}\textbf{9.13} & 75.56 \\
 & pre-train w/ PSC & \cellcolor{red!10}\textbf{23.29} & \cellcolor{red!10}\textbf{80.14} & \cellcolor{red!10}\textbf{22.07} & \cellcolor{red!10}\textbf{81.02} & \cellcolor{red!10}\textbf{10.77} & \cellcolor{red!10}\textbf{80.40} & 8.88 & \cellcolor{red!10}\textbf{78.20} \\ \midrule \midrule
\multirow{6}{*}{Structure} & GAT & 22.11 & 83.65 & 21.56 & 84.68 & 10.70 & 83.88 & 9.40 & 83.90 \\
 & pre-train w/ PSC & \cellcolor{blue!10}\textbf{24.26} & 84.10 & \cellcolor{blue!10}\textbf{23.78} & 85.51 & 11.14 & 84.52 & 10.62 & 84.74 \\ \cmidrule(r){2-10} 
 & GCN & 22.37 & 83.69 & 22.09 & 85.02 & 10.12 & 85.47 & 9.58 & 85.35 \\
 & pre-train w/ PSC & 24.12 & 84.53 & 23.52 & \cellcolor{blue!10}\textbf{85.88} & 11.78 & \cellcolor{blue!10}\textbf{85.95} & 10.62 & \cellcolor{blue!10}\textbf{85.80} \\ \cmidrule(r){2-10} 
 & SAGE & 22.73 & \cellcolor{blue!10}\textbf{85.10} & 21.95 & 84.33 & 11.95 & 84.94 & 10.84 & 85.63 \\
 & pre-train w/ PSC & 23.64 & 84.83 & 23.49 & 85.86 & \cellcolor{blue!10}\textbf{12.70} & 85.63 & \cellcolor{blue!10}\textbf{11.20} & 85.51 \\ \midrule \midrule
\multirow{4}{*}{\begin{tabular}[c]{@{}c@{}}Sequence \& Structure\end{tabular}} & Concatenation & 23.86 & 84.58 & 23.12 & 85.34 & 9.06 & 82.79 & 8.52 & 82.79 \\
 & pre-train w/ PSC & 25.42 & 84.95 & 24.67 & \cellcolor{green!10}\textbf{86.12} & \cellcolor{green!10}\textbf{11.03} & \cellcolor{green!10}\textbf{86.41} & \cellcolor{green!10}\textbf{11.65} & 85.29 \\ \cmidrule(r){2-10} 
 & Cross-Interaction & 24.02 & 83.57 & 23.55 & 84.68 & 11.80 & 85.56 & 10.89 & 84.37 \\
 & pre-train w/ PSC & \cellcolor{green!10}\textbf{26.56} & \cellcolor{green!10}\textbf{85.33} & \cellcolor{green!10}\textbf{25.12} & 85.72 & 12.46 & 85.82 & 11.46 & \cellcolor{green!10}\textbf{86.19} \\ \bottomrule
 
\end{tabular}}
\end{center}
\end{table*}
\begin{table*}[!tbp]
\begin{center}
\caption{Performance comparison of \textit{CPI strength prediction} with Root Mean Square Error (RMSE, lower is better) and Pearson correlation coefficients (PPCs, higher is better) as evaluation metrics under four data splits on the Karimi dataset, where three inference settings are evaluated, and the best metrics for each inference setting are marked by different colors.}
\label{tab:A2}
\resizebox{0.9\textwidth}{!}{
\begin{tabular}{clcccccccc}
\toprule
\multirow{2}{*}{\begin{tabular}[c]{@{}c@{}}\textbf{Inference} \textbf{Setting}\end{tabular}} & \multicolumn{1}{c}{\multirow{2}{*}{\textbf{Methods}}} & \multicolumn{2}{c}{\textbf{Seen-Both}} & \multicolumn{2}{c}{\textbf{Unseen-Comp}} & \multicolumn{2}{c}{\textbf{Unseen-Prot}} & \multicolumn{2}{c}{\textbf{Unseen-Both}} \\ \cmidrule(r){3-4}  \cmidrule(r){5-6} \cmidrule(r){7-8} \cmidrule(r){9-10}
 & \multicolumn{1}{c}{} & \textbf{RMSE} $\downarrow$ & \textbf{PCCs} $\uparrow$ & \textbf{RMSE} $\downarrow$ & \textbf{PCCs} $\uparrow$ & \textbf{RMSE} $\downarrow$ & \textbf{PCCs} $\uparrow$ & \textbf{RMSE} $\downarrow$ & \textbf{PCCs} $\uparrow$ \\ \midrule
\multirow{6}{*}{\quad Sequence \quad} & HRNN & 1.56 & 0.67 & 1.48 & 0.67 & 1.66 & 0.54 & 1.75 & 0.54 \\
 & pre-train w/ PSC & 1.48 & \cellcolor{red!10}\textbf{0.70} & 1.37 & 0.72 & \cellcolor{red!10}\textbf{1.54} & 0.52 & 1.59 & \cellcolor{red!10}\textbf{0.58} \\ \cmidrule(r){2-10} 
 & LSTM & 1.58 & 0.66 & 1.47 & 0.64 & 1.62 & 0.53 & 1.67 & 0.53 \\
 & pre-train w/ PSC \quad & 1.49 & 0.69 & 1.38 & 0.72 & 1.56 & \cellcolor{red!10}\textbf{0.54} & 1.57 & 0.57 \\ \cmidrule(r){2-10} 
 & Bi-LSTM & 1.62 & 0.60 & 1.45 & 0.67 & 1.60 & 0.50 & 1.62 & 0.53 \\
 & pre-train w/ PSC & \cellcolor{red!10}\textbf{1.46} & 0.69 & \cellcolor{red!10}\textbf{1.35} & \cellcolor{red!10}\textbf{0.73} & 1.55 & 0.53 & \cellcolor{red!10}\textbf{1.55} & 0.57 \\ \midrule \midrule
\multirow{6}{*}{Structure} & GAT & 1.58 & 0.65 & 1.52 & 0.65 & 1.73 & 0.51 & 1.80 & 0.49 \\
 & pre-train w/ PSC & 1.53 & \cellcolor{blue!10}\textbf{0.66} & 1.43 & 0.67 & 1.52 & 0.56 & 1.66 & 0.53 \\ \cmidrule(r){2-10} 
 & GCN & 1.64 & 0.59 & 1.47 & 0.64 & 1.71 & 0.52 & 1.64 & 0.54 \\
 & pre-train w/ PSC & \cellcolor{blue!10}\textbf{1.52} & \cellcolor{blue!10}\textbf{0.66} & \cellcolor{blue!10}\textbf{1.39} & \cellcolor{blue!10}\textbf{0.70} & 1.53 & 0.55 & \cellcolor{blue!10}\textbf{1.58} & 0.55 \\ \cmidrule(r){2-10} 
 & SAGE & 1.61 & 0.61 & 1.48 & 0.65 & 1.62 & 0.52 & 1.69 & 0.51 \\
 & pre-train w/ PSC & 1.55 & 0.64 & 1.42 & 0.68 & \cellcolor{blue!10}\textbf{1.48} & \cellcolor{blue!10}\textbf{0.57} & \cellcolor{blue!10}\textbf{1.58} & \cellcolor{blue!10}\textbf{0.57} \\ \midrule \midrule
\multirow{4}{*}{\begin{tabular}[c]{@{}c@{}}Sequence \& Structure\end{tabular}} & Concatenation & 1.55 & 0.66 & 1.44 & 0.69 & 1.61 & 0.49 & 1.65 & 0.51 \\
 & pre-train w/ PSC & \cellcolor{green!10}\textbf{1.42} & \cellcolor{green!10}\textbf{0.71} & 1.31 & 0.73 & 1.47 & 0.57 & \cellcolor{green!10}\textbf{1.52} & \cellcolor{green!10}\textbf{0.60} \\ \cmidrule(r){2-10} 
 & Cross-Interaction & 1.49 & 0.68 & 1.36 & 0.71 & 1.50 & 0.56 & 1.62 & 0.55 \\
 & pre-train w/ PSC & 1.43 & 0.70 & \cellcolor{green!10}\textbf{1.30} & \cellcolor{green!10}\textbf{0.74} & \cellcolor{green!10}\textbf{1.42} & \cellcolor{green!10}\textbf{0.59} & 1.55 & 0.58 \\ \bottomrule
 
\end{tabular}}
\end{center}
\end{table*}
